# Supplementary material for: Sequential Cooperative Energy and Time-Optimal Lane Change Maneuvers for Highway Traffic
Source: arXiv:2203.17102 source file (2022-03-31)
Supplement: Supplementary file 1 [file appendix.tex]

\begin{algorithm}[h]
    \caption{Optimal Longitudinal Maneuver}
    \SetKwInOut{Input}{input}
    \SetKwInOut{Output}{output}
    \Input{Initial Conditions $x_i(t_0),v_i(t_0)\coloneqq\{i|i\in S(t)\}$,  $x_U(t_0),x_U(t_0)$, and $x_C(t_0),x_C(t_0)$, Relaxation Constant $\lambda_{t_f}$,\\Free Flow speed $v_{d}$, Maximum Time $T_{th}$,\\ Maximum Disturbance $D_\text{th}$} 
    \Output{Optimal Longitudinal Trajectories $u_i^*(t) \coloneqq \{u_i^*(t)|i\in S(t^*_f), t\in \lbrack t_0,t^*_f\rbrack$\}}
    \SetKwBlock{Beginn}{beginn}{ende}
    \Begin{
        %State
        % $\text{count}\leftarrow 1$, 
        $(i^*,i^*+1)\leftarrow \emptyset$ \\ 
        %State
        $t^*_f,x_c(t_f^*),u_c^*\leftarrow$ Compute OCP for CAV C  \eqref{eq:cav_c_objective_simplified}\\
        % \While{$S^*=\emptyset \wedge \text{count}\leq 5$}{
        \While{$i^*=\emptyset \wedge t_f\leq T_{th}$}{
            %State
            $S(t^*_f)\leftarrow$ Compute Relevant CAV Set \eqref{eq9:subset_definition}\\
            $i=1$, $N=|S(t^*_f)|$, $\Hat{D} = \emptyset$\\
            \For{$i=1$ to $N-1$}{
                %State
                $x_i(t^*_f),x_{i+1}(t^*_f)\leftarrow$ Compute Terminal Positions \eqref{eq:terminal_position}\\
                % State
                $D_{i,i+1}\leftarrow$ Compute Disruption \eqref{eq:disruption}\\
                % State
                \If{$D_{i,i+1}\leq D_\text{th}$}{
                    $\Hat{D}\leftarrow$ Append tuple $\left\langle i, D_{i,i+1} \right\rangle$\\
                } %end \If{$f_{i,i+1}=1$}
            }%end For $i\in S(t_f)$
            $(i^*,i^*+1)\leftarrow$ Compute optimal CAV Set \eqref{eq:optimal_collaboration_pair}\\
            \eIf{$(i^*,i^*+1)\neq\emptyset$}{
                $u_i^*,u_{i+1}^*\leftarrow$ Compute optimal trajectories for $i^*$ and $i^*+1$ \eqref{eq:cav_i_problem}\\
                break
            } %end if
            {%else
                $t'_f\leftarrow$ Relax Terminal Time $t^*_{f}\lambda_{t_f}$\\
                $x_c(t_f'),u_c^*\leftarrow$ Relaxed OCP  \eqref{eq:cav_c_relaxedTime}\\
                $\text{count}+1$
            }
        }% end while
    }
    \label{alg1:Optimal_longitudinal_lane-change}
    % \vspace*{-\baselineskip}
    % \vspace*{-\baselineskip}
\end{algorithm}
